# Supplementary material for: G-PATE: Scalable Differentially Private Data Generator via Private Aggregation of Teacher Discriminators
Source: arXiv:1906.09338 source file (2021-12-30)
Supplement: Supplementary file 1 [file analysis.tex]

\section*{Appendix C. Privacy Analysis}
In this section, we analyze the data dependent privacy budget $\varepsilon$ for training \name{}. 

For completeness of the paper, we recall the Confident-GNMax aggregator proposed in scalable PATE~\cite{papernot2018scalable} in Algorithm~\ref{algo:gnmax}.
\input{algorithms/GNMax.tex}

We start with recalling the definition of differential privacy (DP), R\'enyi differential privacy (RDP), and some of their properties. 

\begin{definition}[$(\varepsilon, \delta)$-Differential Privacy]
A randomized algorithm $\mathcal{M}$ with domain $\mathbb{N}^{|\mathcal{X}|}$ is $(\varepsilon,\delta)$-differentially private if for all $\mathcal{S} \subseteq \Range{\mathcal{M}}$ 
and for any neighboring datasets $D$ and $D'$:
\begin{equation*}
    \Pr[\mathcal{M}(D) \in \mathcal{S}] \leq \exp(\varepsilon)\Pr[\mathcal{M(D')\in \mathcal{S}}] + \delta.
\end{equation*}
\end{definition}

\begin{definition}[$(\lambda, \varepsilon)-$RDP]
A randomized mechanism $\mathcal{M}$ is said to guarantee $(\lambda, \varepsilon)$-RDP with $\lambda \geq 1$ if for any neighboring datasets $D$ and $D'$,
\begin{equation*}
    D_{\lambda}\left(\mathcal{M}(D) \| \mathcal{M}\left(D^{\prime}\right)\right)=\frac{1}{\lambda-1} \log \mathbb{E}_{x \sim \mathcal{M}(D)}\left[\left(\frac{\mathbf{P} \mathbf{r}[\mathcal{M}(D)=x]}{\mathbf{P r}\left[\mathcal{M}\left(D^{\prime}\right)=x\right]}\right)^{\lambda-1}\right] \leq \varepsilon.
\end{equation*}
\end{definition}

RDP allows tighter composition of heterogeneous mechanisms and can be converted to $(\varepsilon,\delta)$-differential privacy~\cite{mironov2017renyi}.

\begin{theorem}[Composition of RDP~\cite{mironov2017renyi}]
\label{theorem:rdpc}
If a mechanism $\mathcal{M}$ consists of a sequnce of $\mathcal{M}_1, \dots, \mathcal{M})k$ such that for any $i \in [k]$, $\mathcal{M}_i$ guarantees $(\lambda, \varepsilon_i)$-RDP, then $\mathcal{M}$ guarantees $(\lambda, \sum_{i=1}^k\varepsilon_i)$-RDP.
\end{theorem}

\begin{theorem}[From RDP to DP~\cite{mironov2017renyi}]
\label{theorem:rdp-dp}
If a mechanism $\mathcal{M}$ guarantees $(\lambda, \varepsilon)$-RDP, then $\mathcal{M}$ guarantees $(\varepsilon + \frac{\log 1/\delta}{\lambda-1}, \delta)$-differential privacy for any $\delta \in (0,1)$.
\end{theorem}

We first analyze the privacy guarantee for a single query to the Confident-GNMax aggregator. A Confident-GNMax aggregator consists of two steps. First, it computes the noisy maximum votes
\begin{equation*}
    M_1 = \max_i\{n_j(x)\} + \mathcal{N}(0, \sigma_1^2).
\end{equation*}
Then, it uses the GNMax mechanism to select the output with most votes:
\begin{equation*}
    M_2 = \arg\max\{n_j(x) + \mathcal{N}(0, \sigma_2^2)\}.
\end{equation*}

Theorem~\ref{theorem:gnmax} presents the data dependent privacy guarantee for the GNMax aggregator $M_2$. 

\begin{theorem} [Data Dependent Privacy Bound for GNMax Mechanism~\cite{papernot2018scalable}]
\label{theorem:gnmax}
If the top three vote counts are $n_1 > n_2 > n_3$ and $n_1 - n_2, n_2 - n_3 \gg \sigma$, then the mechanism GNMax with Gaussian of variance $\sigma^2$ satisfies $(\lambda, \exp(-2\lambda/\sigma^2)/\lambda$-RDP for $\lambda=(n_1-n_2)/4$.
\end{theorem}

Additionally, we analyze the data independent privacy guarantee for the noisy maximum votes mechanism $M_1$. 
\begin{theorem}
\label{theorem:thresh}
The maximum noisy votes mechanism with Gaussian of variatnce $\sigma^2$ guarantees $(\lambda, \lambda/2\sigma^2)$-RDP for all $\lambda > 1$.
\end{theorem}
\begin{proof}
Since each teacher model may cause the maximum number of votes to change at most by 1. The maximum noisy votes mechanism is equivalent to a Gaussian mechanism with sensitivity 1. Hence, it satisfies $(\lambda, \lambda/2\sigma^2)$-RDP~\cite{mironov2017renyi}.
\end{proof}

Since a student generator can only access information about the sensitive data through the Confident-GNMax aggregator, the privacy budget for training the student generator is the composition of privacy budgets across multiple runs of the aggregator.
