# Supplementary material for: G-PATE: Scalable Differentially Private Data Generator via Private Aggregation of Teacher Discriminators
Source: arXiv:1906.09338 source file (2021-12-30)
Supplement: Supplementary file 2 [file algo.tex]

% \section*{Appendix. Algorithm}
\subsection{Algorithm for Training the Student Generator}
\label{appendix:algorithm}
\input{algorithms/trainGen.tex}
