# Supplementary material for: G-PATE: Scalable Differentially Private Data Generator via Private Aggregation of Teacher Discriminators
Source: arXiv:1906.09338 source file (2021-12-30)
Supplement: Supplementary file 3 [file appendix-main.tex]

% \documentclass{article}
% \input{macros.tex}

% \title{Supplementary Material for Scalable Differentially Private Generative Student Model via PATE}

% \begin{document}
% \date{}
% \maketitle

% \input{appendix/appendix.tex}

% \newpage
% \bibliographystyle{plain}
% \bibliography{main} 

% \end{document}
