# Supplementary material for: G-PATE: Scalable Differentially Private Data Generator via Private Aggregation of Teacher Discriminators
Source: arXiv:1906.09338 source file (2021-12-30)
Supplement: Supplementary file 4 [file appendix.tex]

\appendix
% \section{Appendix}
% \input{appendix/algo.tex}
\input{appendix/kaggle.tex}
\input{appendix/images.tex}
\input{appendix/nonprivate.tex}
\input{appendix/analysis-new.tex}
\input{appendix/params.tex}
\input{appendix/visual.tex}
\input{appendix/running_time.tex}
\input{appendix/dp_proof.tex}
