# Supplementary material for: G-PATE: Scalable Differentially Private Data Generator via Private Aggregation of Teacher Discriminators
Source: arXiv:1906.09338 source file (2021-12-30)
Supplement: Supplementary file 5 [file teachers.tex]

\subsection{Analysis on the Number of Teacher Models on Fashion-MNIST}
\label{appendix:teachers}

Table~\ref{tab:teachers} presents the 10-class classification accuracy for models trained on synthetic data produced by \name{} with different number of teachers on Fashion-MNIST dataset. For 2000 teachers, we set $\sigma_1=1700, \sigma_2=1000$ and use 5 project dimensions for random projection. We use 10 project dimensions for both 3000 and 4000 teachers. We set $\sigma_1=2000, \sigma_2=1000$ for 3000 teachers, and  $\sigma_1=3000, \sigma_2=1000$ for 4000 teachers. It is shown that more teacher models will help improve the data utility while 4000 teacher models have already achieved satisfiable results. 

\begin{table}[h]
\centering
\begin{tabular}{l|lll}
\toprule
\textbf{Number of Teacher Models} & 2000 & 3000 & 4000 \\ \midrule
% \textbf{MNIST} & 0.4240 & 0.5218 & \textbf{0.5631} \\ 
\textbf{Classification Accuracy} & 0.3997 & 0.4874 & \textbf{0.5174} \\
\bottomrule
\end{tabular}
% \vspace{7pt}
\caption{\textbf{Analysis on the Number of Teacher Models.} The best results are bolded. }
\label{tab:teachers}
\end{table}

% \yunhui{Add analysis on results in the table}
% \input{tables/projection.tex}
